# Supplementary material for: Inference for extreme earthquake magnitudes accounting for a time-varying measurement process
Source: arXiv:2102.00884 source file (2021-02-01)
Supplement: Supplementary file 1 [file 92_appendix_sampling_z.tex]

\section{Sampling standardised threshold exceedances} \label{app:sampling_z}

 This appendix describes how to sample a vector $\tilde{\bm{z}}$ of unrounded threshold exceedances transformed to have a common Exp(1) marginal distribution. This uses a single bootstrap estimate of the underlying GPD parameters $\hat{\bm{\theta}}$, the n-vector of rounded observations $\bm{x}$ and the corresponding threshold vector $\bm{v}$. The process is described for sampling a single vector $\tilde{\bm{z}}$ and is formalised in Algorithm~\ref{alg:simulate_standardised_exceedances}. 
 
 It is unknown which, if any, of the borderline values $\{x_j \in \bm{x}: |x_j - v_j| < \delta$\} correspond to unrounded values that exceed the modelling threshold. The first step in sampling $\tilde{\bm{z}}$ is therefore to sample the set $I$ of events that are threshold exceedances. This is done by simulating independent Bernoulli trials for each event $j = 1, \dots, n$ with success probabilities $w_j = \Pr(Y_i > v_i | x_i, \hat{\bm{\theta}})$ as defined in equation~\eqref{eqn:rounded_gpd_weights}.  The vector $\tilde{\bm{z}}$ will therefore have a randomly sampled length $\tilde n = |I| \leq n$, where the distribution of $\tilde n$ depends on $\bm{x}, \bm{v}$ and $\hat{\bm{\theta}}$.

 The unrounded magnitude values for events sampled to be in $I$ are then simulated from their conditional distribution given their rounded values, the estimated GPD parameters and that they are threshold exceedances. Letting $F$ be the GPD distribution function, the required conditional distribution function of $Y_j| x_j, \bm{\theta}, Y_j \geq v_j$ is given by: 
\begin{equation} \label{eqn:unrounded_conditional_distribution}
    G_{Y_j| x_j, \bm{\theta}, Y_j \geq v_j}(y) = 
    \left\{
    \begin{array}{cr}
        0 & \text{ for } y < b_j,  \\
        \frac{F(y - u;\bm{\theta}) - F(b_j - u; \bm{\theta})}{F(x_j + \delta - u; \bm{\theta}) - F(b_j - u ; \bm{\theta})} & \text{ for } b_j \leq y \leq x_j + \delta, \\
        1 & \text{ for } y > x_j + \delta,
    \end{array}
    \right.
\end{equation}
where $j \in I$ and $b_j = \max(x_j - \delta, v_j)$  is the smallest value above the modelling threshold that results in a rounded value of $x_j$. The sampled values are combined to create the $\tilde{n}$-vector $\tilde{\bm{y}}$ of sampled unrounded threshold exceedances. The probability integral transform is then used to give each of element of $\tilde{\bm{y}}$ to have an Exp(1) marginal distribution under the fitted GPD model. This results in the vector $\tilde{\bm{z}}$ of standardised, sampled values for the observed exceedances of the modelling threshold $v(\tau)$. 
 
To construct confidence intervals for PP- or QQ-plots and to calculate expected distance metrics, $\tilde{\bm{z}}$ is sampled for each of a large number $k$ of bootstrap parameter estimates $\hat{\bm{\theta}}^{(1)}, \dots, \hat{\bm{\theta}}^{(k)}$. This gives a set of sampled vectors $\tilde{\bm{z}}^{(1)}, \dots,\tilde{\bm{z}}^{(k)}$ of lengths $\tilde{n}^1,\dots,\tilde{n}^k$. Uncertainty in the estimated GPD parameters, the size of the exceedance set and the values of unrounded exceedances are each represented across these realisations of $\bm{z}$.

\begin{algorithm}[htbp]
\SetAlgoLined
    \SetKwInOut{Input}{input}
    \SetKwInOut{Output}{output}
    \Input{A bootstrap estimate of the GPD parameters $\hat{\bm{\theta}} = (\hat\sigma, \hat\xi)$, an $n$-vector of rounded observed values $\bm{x}$ and the corresponding thresholds $\bm{v}$.}
    \Output{A vector $\tilde{\bm{z}}$ of length $\tilde n \leq n$ of sampled unrounded values, transformed to have an Exp(1) distribution under the fitted model.}
  
    \For{$j = 1$ \KwTo $n$}{
    calculate $w_j = \text{Pr}(Y_j > v_j | x_j, \hat{\bm{\theta}})$, the probability that each rounded observation corresponds to an unrounded value on $A_v$, as in equation \eqref{eqn:rounded_gpd_weights}\;
    }
    Generate $n$ independent Uniform[0,1] random variables $u_1,\dots,u_n$ \;
    Sample the indexing set for events that are on $A_v$, $I = \{j \in (1,\dots,n) : u_j \leq w_j\}$ and let $\tilde n = |I|$ \;
    Store the elements of $I$ in the vector $\bm{\nu}= (\nu_1, \dots, \nu_{\tilde n})$ and
    initialise $\bm{\tilde y}$ and $\bm{\tilde z}$ as vectors of length $\tilde{n}$\;
    \For{$j = 1$ \KwTo $\tilde n$}{
        Let $a = \nu_{j}$ \;
        Sample the $j^{\text{th}}$ unrounded exceedance $\tilde{y}_{j}$ from its conditional distribution $G_{Y_a | x = x_a,\bm{\theta} = \hat{\bm{\theta}},  Y_a \geq v_a,} (y)$ as in equation \eqref{eqn:unrounded_conditional_distribution} \;
        Let $\hat{\bm{\theta}}_{v_a} = (\hat \sigma - \hat\xi(v_a - u), \hat\xi)$ be the GPD parameters for exceedances of $v_a$\;
        Transform $\tilde{y}_j$ onto  Exp(1) margins under the fitted model by letting $F$ be the GPD distribution function \eqref{eq:gpd_distn_function} and setting 
        $$\tilde{z}_j = - \log \left[ 1 - F\left(y_j - v_{a}; \hat{\bm{\theta}}_{v_a} \right)\right].$$
    }

 \caption{Simulation of standardised threshold exceedance sets}
 \label{alg:simulate_standardised_exceedances}
\end{algorithm}

\textbf{The following text was cut from main document and explains construction of modified PP and QQ plots.} 

To overcome these challenges we simulate the unrounded threshold exceedance values $\tilde{\bm{y}} \subseteq \bm{y}$, given the rounded values $\bm{x}$, modelling threshold $\bm{v}$ and estimated GPD parameters $\hat{\bm{\theta}}$. To do this, we first sample the set of observations $I \subseteq \{1, \dots, n\}$ that exceed the threshold given $\bm{x}, \bm{v}$ and $\hat{\bm{\theta}}$. We then sample the unrounded values for these exceedances from their conditional distributions, again given $\bm{x}, \bm{v}$ and $\hat{\bm{\theta}}$. 

The sampled vector of unrounded threshold exceedances $\tilde{\bm{y}}$  is of length $\tilde{n} \leq n$ and each element of $\tilde{\bm{y}}$ has a distribution within the GPD family, but the elements may not have the same GPD parameters due to their different modelling thresholds. We ensure an identical distribution for the sampled unrounded exceedances $\tilde{\bm{y}}$ by transforming each to have Exponential(1) marginal distribution. This results in a vector $\tilde{\bm{z}}$ of $\tilde{n} \leq n$ simulated threshold exceedance values on shared exponential margins. The process of simulating $\tilde{\bm{z}}$ is described fully in Appendix \ref{app:sampling_z}. From this vector, a standard QQ- or PP- plot may be constructed and tolerance intervals for an exponential data set of the same size added.

 Exponential margins were chosen for $\tilde{\bm{z}}$ because this is the central distribution within the GPD family and it follows the precedent set by \citet{heffernan2001extreme}. This choice impacts only the QQ-plot and alternative marginal distributions could be used, with the PP-plot being the special case of uniform margins.

Using only one simulated vector $\tilde{\bm{z}}$ to construct PP- or QQ-plots ignores the uncertainty in the sampled probability or quantile values. These have been sampled based on the estimated GPD parameters, the sampled exceedance set and the sampled unrounded values - each of which presents a source of uncertainty. To represent this uncertainty in the plots, $\tilde{\bm{z}}$ can be simulated for each of a set of $k$ bootstrap parameter estimates, $\hat{\bm{\theta}}^{(1)}, \dots, \hat{\bm{\theta}}^{(k)}$, where the exceedance sets and unrounded values are sampled separately for each bootstrap estimate. The resulting vectors $\tilde{\bm{z}}^{(1)}, \dots, \tilde{\bm{z}}^{(k)}$ of lengths $\tilde{n}^{(1)}, \dots, \tilde{n}^{(k)}$ can then be used to construct Monte Carlo confidence intervals for each probability or quantile. Given the vectors $\tilde{\bm{z}}^{(1)}, \dots, \tilde{\bm{z}}^{(k)}$, tolerance intervals on probabilities or quantiles are easily adjusted to account for uncertainty in the number of exceedances. Comparing these to their respective confidence intervals allows a distributional assessment to be made that accounts for the GPD parameters having been estimated and for the exceedance set and unrounded values being unknown.  When the confidence and tolerance intervals do not overlap, it suggests that the distribution of the rounded exceedances is not coherent with the fitted GPD model.
