# Supplementary material for: Inference for extreme earthquake magnitudes accounting for a time-varying measurement process
Source: arXiv:2102.00884 source file (2021-02-01)
Supplement: Supplementary file 12 [file 93_appendix_return_level_plots.tex]

\section{Return level plots with variable threshold} 
\label{app:return_level_bootstrap}

Return level plots allow defensive structures to be designed so that they are  expected to be overcome only once in every $m$ events. In the case of i.i.d event magnitudes, the $m$-event return level is the $p = 1 - 1/m$ quantile of the size distribution and is written $x_{p}$. 

For time series data this can be easily estimated. A threshold $u$ is selected, a GPD is fit above this threshold and $q_u$, the probability that each observation exceeds $u$, is estimated. This gives parameter estimates $(\hat \sigma_u, \hat\xi, \hat q_u)$. The return level $x_p$ can be written as a closed form function of these parameters and so a point estimate and confidence interval on $x_p$ may be easily obtained. When $x_p \geq u$, 
\begin{equation}
    x_p = \left\{
    \begin{array}{ll}
    q_u \left[ u + \frac{\sigma_u}{\xi}\left({p}^{-\xi} - 1\right)\right] & \text{ if } \xi \neq 0, \\
    q_u \left[ u - \sigma_u \log(p)\right] & \text{ if } \xi = 0.
    \end{array}
    \right.
\end{equation}
Since we do not have complete data at small magnitudes we will instead calculate \textit{conditional} $m$-event return level above the threshold $u$. This the the event magnitude that is expected to be exceeded by only one in every $m$ events that have magnitude of at least $u$. Using the conditional $m$-event return level $x_{p,u} = x_p / q_u$ means that it is not necessary to estimate $q_u$ using incomplete data.  

Suppose we have fitted a GPD above threshold $u$ to obtain $(\hat \sigma_u, \hat \xi)$ and want to calculate conditional return levels above a higher threshold $v>u$. Letting $\zeta = \Pr(X \geq v|X \geq u)$, the conditional $m_1,\dots ,m_j$-event return levels above $v$ are equivalent to estimating the  $\frac{m_1}{\zeta},\dots,\frac{m_j}{\zeta}$-event levels above $u$. Obtaining a point estimate of these is simple since: 
\begin{equation}
    x_{p,v} = x_{\zeta p, u} \left\{
    \begin{array}{ll}
    u + \frac{\sigma_u}{\xi}\left({(\zeta p)}^{-\xi} - 1\right) & \text{ if } \xi \neq 0, \\
     u - \sigma_u \log(\zeta p) & \text{ if } \xi = 0.
    \end{array}
    \right.
\end{equation}

To construct the conditional return-level plot in Figure~\ref{fig:simple_return_level_plot} we display the return level against the log return period. For clarity we choose to leave this displayed for the latent process rather than the observed, rounded values. 

\begin{figure}[htbp]
    \centering
    \includegraphics[width = 0.5\textwidth]{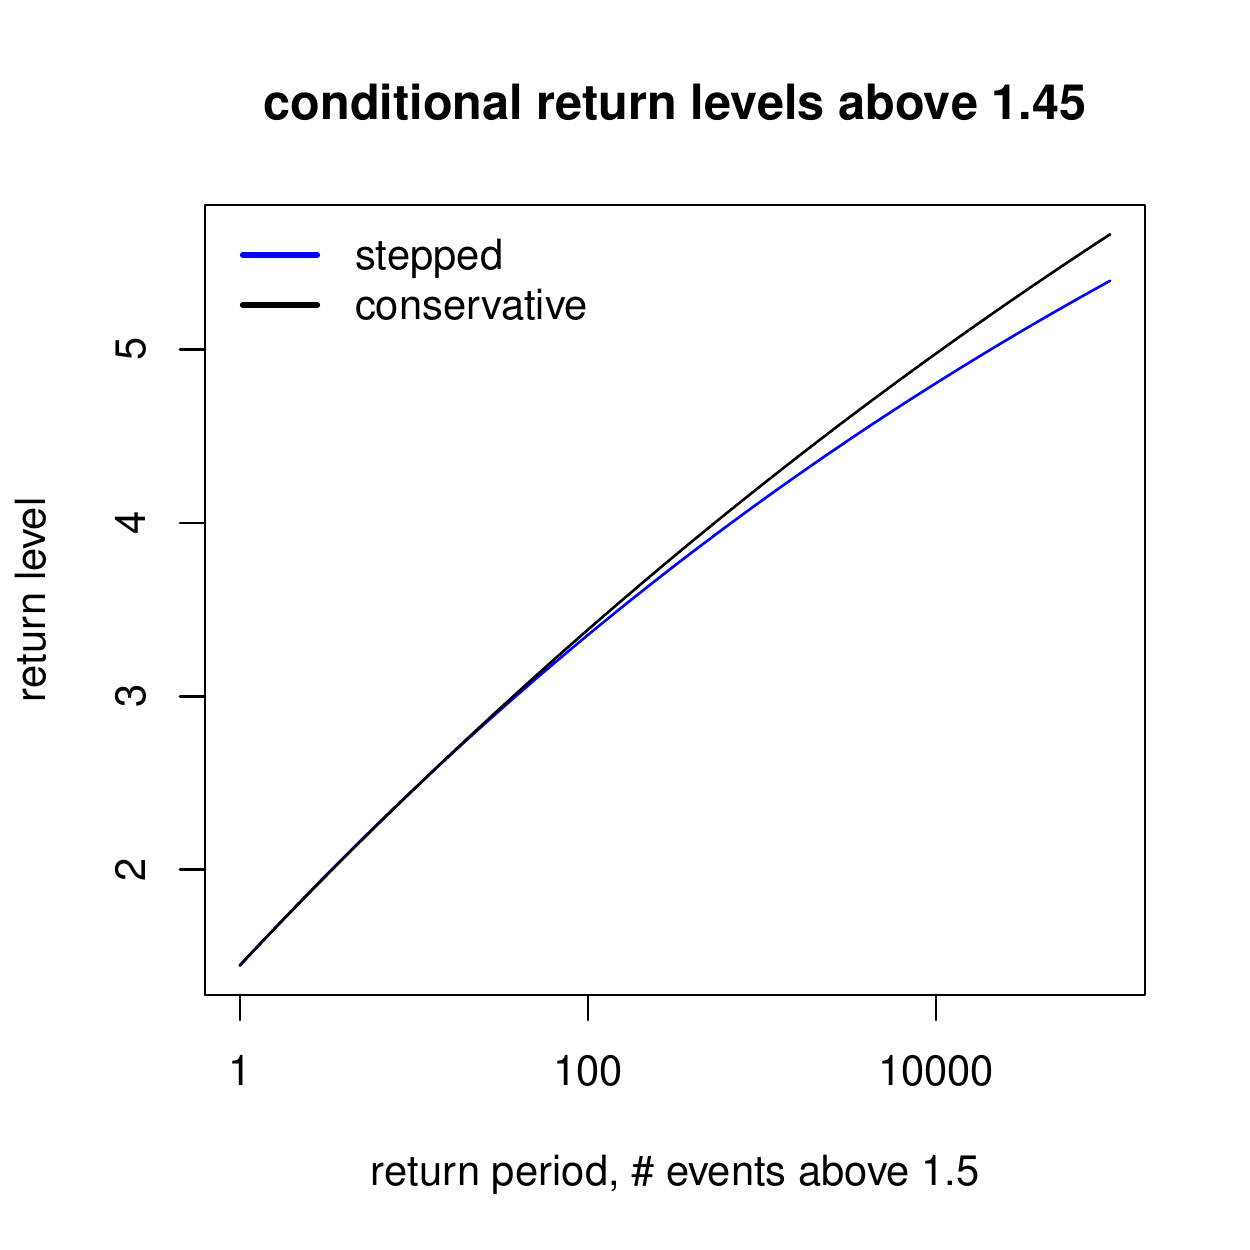}
    \caption{Point estimates of conditional return levels above magnitude 1.45 using a conservative threshold of $u=1.45$ and a stepped threshold $u_1 = 1.45, u_2 = 1.05$.}
    \label{fig:simple_return_level_plot}
\end{figure}

\subsection{Parametric bootstrap confidence intervals for conditional return levels.} 
\textbf{Update to avoid repetition from earlier appendix and later adapt to continuous threshold.}

 It is important to show confidence intervals on the estimated return levels, particularly because return levels become increasingly uncertain as the return period increases. We choose to use a parametric bootstrap approach as a simple way to incorporate the effects of rounding and a variable threshold.  

\begin{figure}[htbp]
    \centering
    \includegraphics[width = 0.8\textwidth]{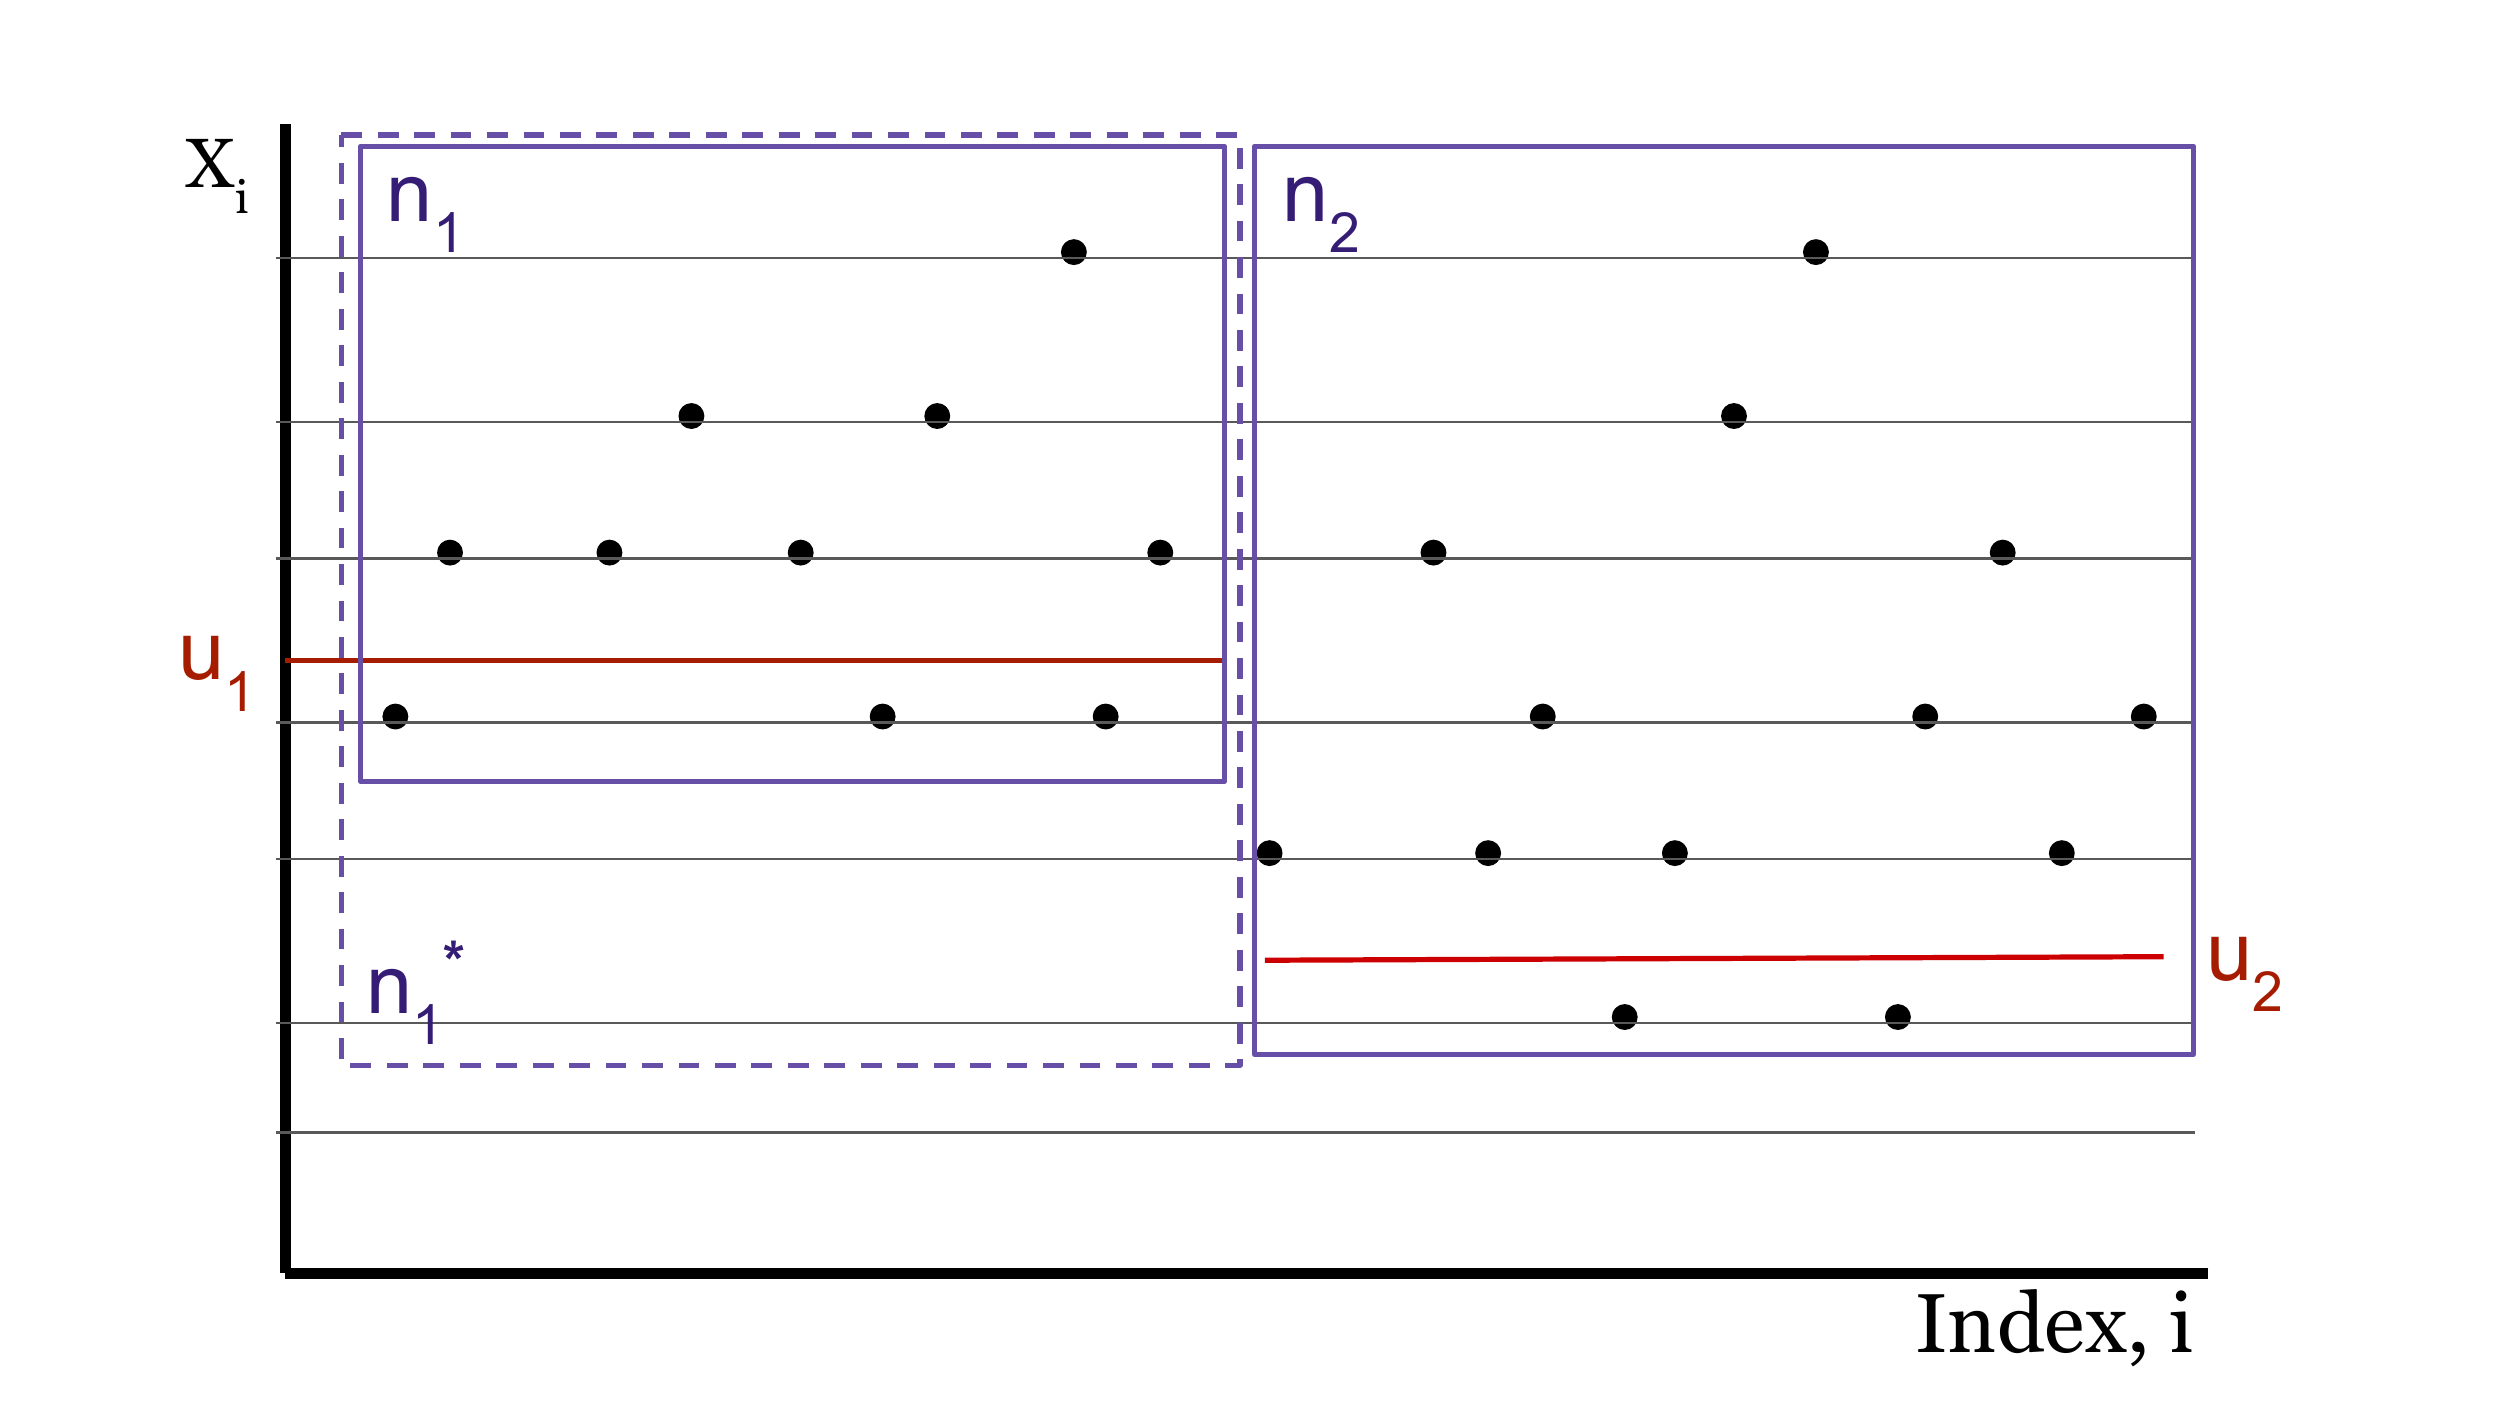}
    \caption{Illustrative rounded data with stepped threshold on latent observations, decreasing from $u_1$ to $u_2$. The observation count at each of the thresholds is $n_1$ and $n_2$. The unknown observation count in the first period is $n_1^* \geq n_1$.
    \textbf{nb:} Depending on the latent threshold value, observations might fall in the first category below the threshold.}
    \label{fig:example_rounded_data_rl_plot}
\end{figure}

The data we are modelling has the same form as the toy example shown in figure \ref{fig:example_rounded_data_rl_plot}. The number of observations $n_1$ seen at the first threshold level $u_1$ is random and depends on the parameters of the underlying distribution above the lower threshold $u_2$. When creating bootstrap datasets we must account for this randomness. 

We must estimate the total number of events $n_1^*$ in the first period that are above the lower threshold $u_2$. Since each event in the first period is above the threshold $u_1$ with probability $\zeta$, it follows that $ N_1^* \sim  \text{NegBin}(n_1, \zeta)$
\vspace{1cm}

\hrule
\textit{To construct a $(1 - \alpha)\%$ bootstrap confidence interval on $x_p$:} 
\hrule
\begin{enumerate}
    \item Find the maximum likelihood estimates $(\hat\sigma_{u_2}, \hat \xi)$ from the observed data.
    \item find $\hat \zeta = \Pr(X > u_1 | X > u_2, \hat \sigma_{u_2}, \hat \xi)$.
    \item Initialise a vector $\mathbf{z}$ to store $b$ bootstrap estimates of $x_p$.
    \item \textbf{For} $i = 1,\dots,b$:
    \begin{enumerate}
        \item sample $\tilde n_1^*$ from a $\text{NegBin}(n_1, \hat \zeta)$ distribution.
        \item sample $\tilde n_1$ from a $\text{Bin}(\tilde n_1^*, \hat \zeta)$ distribution and let $\tilde n = \tilde n_1 + n_2$. 
        \item sample observations $y_1,\dots, y_{\tilde n_1}$ from a GPD$_v(\hat\sigma_{u_2} + (u_1-u_2)\hat \xi, \hat \xi)$ distribution and round to the appropriate level. 
        \item sample observations $y_{\tilde n_1 + 1}, \dots , y_{\tilde n}$ from a GPD$_u(\hat \sigma_{u_2}, \hat \xi)$ and round to the appropriate level. 
        \item Obtain maximum likelihood estimates $(\tilde \sigma_{u_2}, \tilde \xi)$ of the stepped, rounded GPD parameters using the simulated catalogue $y$.  
         \item find $\tilde \zeta = Pr(X > u_1 | X > u_2, \tilde \sigma_{u_2}, \tilde \xi)$.
        \item Calculate the desired return level $\tilde x_{p,v}$ from $(\tilde \sigma_{u_2}, \tilde \xi, \tilde \zeta)$. 
        \item set $\mathbf{z}_i = \tilde x_{p,v}$. 
    \end{enumerate}
    \item Take the $\alpha / 2 $ and $(1 - \alpha / 2)$ quantiles of $\mathbf{z}$ as the bootstrap confidence interval on $x_p$.
\end{enumerate}
\hrule

\vspace{1cm} 
Using this bootstrap method for each return level, point-wise confidence intervals can be added to our return level plots. These are shown in figure \ref{fig:return_level_plot}. 

This technique can be extended to a sigmoid threshold. Instead of re-sampling the number above $u_1$, we have to resample the number of points above the sigmoid. The number of unobserved values before each observation is geometrically distributed with threshold dependent expectation. This allows $\tilde n$ to be constructed in a similar way when forming bootstrap samples.
\begin{figure}[htbp]
    \centering
    \includegraphics[width = 0.7\textwidth]{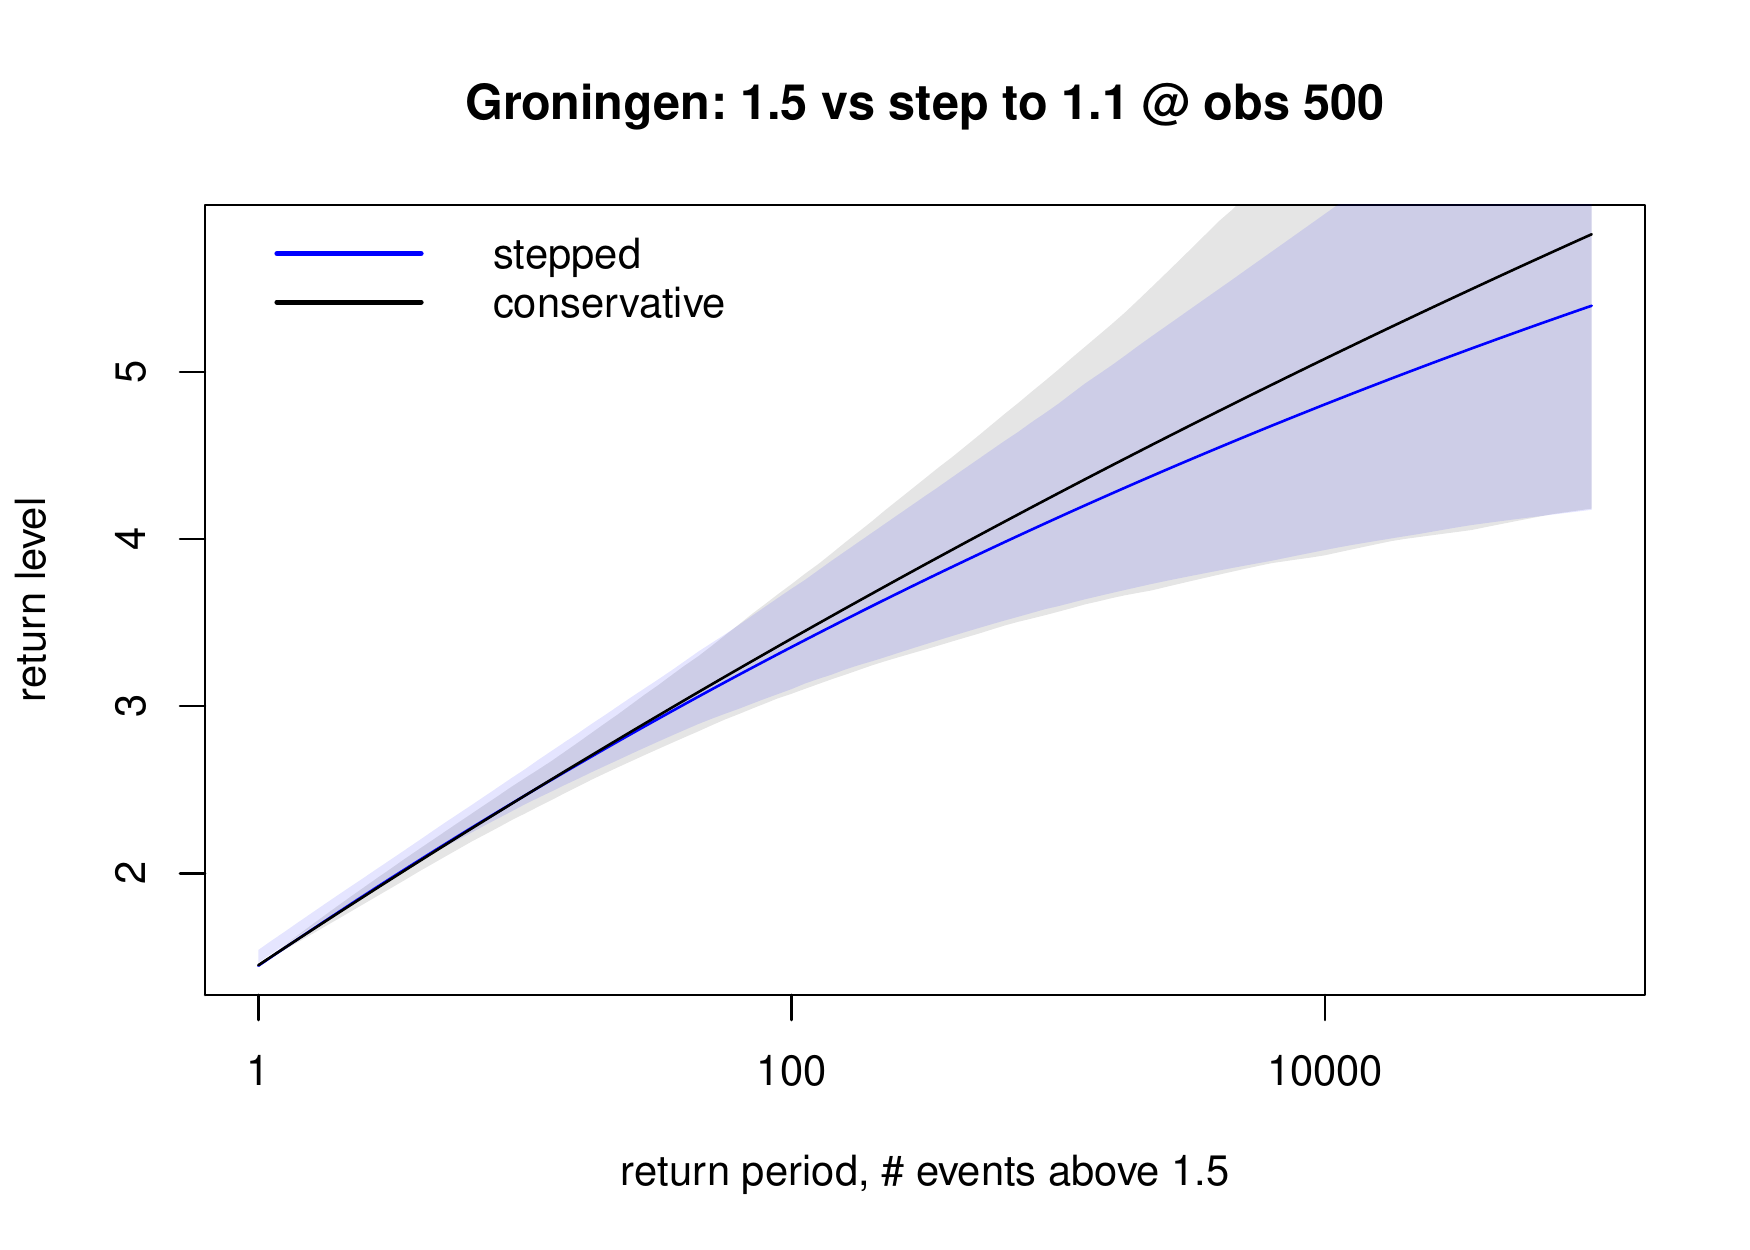}
    \caption{Point-wise estimates and 95\% confidence intervals on conditional return levels above magnitude 1.45. Shown for a conservative threshold of $u=1.45$ and a stepped threshold $u_1 = 1.45, u_2 = 1.05$.}
    \label{fig:return_level_plot}
\end{figure}
